# Supplementary material for: Studies of the resonance structure in $D^{0} \to K^\mp \pi^\pm \pi^\pm \pi^\mp$ decays
Source: arXiv:1712.08609 source file (2018-06-18)
Supplement: Supplementary file 1 [file WS_correlations.tex]

# parameter correlations for D0->K+,pi-,pi-,pi+ amplitude, presented as 
# parameter 1                                      parameter                                          correlation
D0[P]{K*(892)0,rho(770)0}_amp                      D0[P]{K*(892)0,rho(770)0}_phase                    -0.0414102
D0[P]{K*(892)0,rho(770)0}_amp                      D0{K(1)(1270)+,pi-}_amp                            0.6223
D0[P]{K*(892)0,rho(770)0}_amp                      D0{K(1)(1270)+,pi-}_phase                          -0.0773846
D0[P]{K*(892)0,rho(770)0}_amp                      D0{K(1)(1400)+{K*(892)0,pi+},pi-}_amp              0.558922
D0[P]{K*(892)0,rho(770)0}_amp                      D0{K(1)(1400)+{K*(892)0,pi+},pi-}_phase            -0.0836659
D0[P]{K*(892)0,rho(770)0}_amp                      D0{K*(892)0,rho(1450)0}_amp                        0.237661
D0[P]{K*(892)0,rho(770)0}_amp                      D0{K*(892)0,rho(1450)0}_phase                      -0.04129
D0[P]{K*(892)0,rho(770)0}_amp                      D0{K*(892)0,rho(770)0}_amp                         0.318039
D0[P]{K*(892)0,rho(770)0}_amp                      D0{K*(892)0,rho(770)0}_phase                       -0.0730029
D0[P]{K*(892)0,rho(770)0}_amp                      KPi40[FOCUS.I32]{K+,pi-}_amp                       -0.0735834
D0[P]{K*(892)0,rho(770)0}_amp                      KPi40[FOCUS.I32]{K+,pi-}_phase                     0.011858
D0[P]{K*(892)0,rho(770)0}_amp                      PiPi40[kMatrix.pole.1]{pi-,pi+}_amp                0.435517
D0[P]{K*(892)0,rho(770)0}_amp                      PiPi40[kMatrix.pole.1]{pi-,pi+}_phase              -0.0658724
D0[P]{K*(892)0,rho(770)0}_amp                      PiPi40[kMatrix.prod.0]{pi-,pi+}_amp                0.352622
D0[P]{K*(892)0,rho(770)0}_amp                      PiPi40[kMatrix.prod.0]{pi-,pi+}_phase              -0.105993
D0[P]{K*(892)0,rho(770)0}_phase                    D0{K(1)(1270)+,pi-}_amp                            -0.0234316
D0[P]{K*(892)0,rho(770)0}_phase                    D0{K(1)(1270)+,pi-}_phase                          0.471539
D0[P]{K*(892)0,rho(770)0}_phase                    D0{K(1)(1400)+{K*(892)0,pi+},pi-}_amp              0.074841
D0[P]{K*(892)0,rho(770)0}_phase                    D0{K(1)(1400)+{K*(892)0,pi+},pi-}_phase            0.577911
D0[P]{K*(892)0,rho(770)0}_phase                    D0{K*(892)0,rho(1450)0}_amp                        0.000579667
D0[P]{K*(892)0,rho(770)0}_phase                    D0{K*(892)0,rho(1450)0}_phase                      0.213021
D0[P]{K*(892)0,rho(770)0}_phase                    D0{K*(892)0,rho(770)0}_amp                         0.053233
D0[P]{K*(892)0,rho(770)0}_phase                    D0{K*(892)0,rho(770)0}_phase                       0.422214
D0[P]{K*(892)0,rho(770)0}_phase                    KPi40[FOCUS.I32]{K+,pi-}_amp                       0.0229014
D0[P]{K*(892)0,rho(770)0}_phase                    KPi40[FOCUS.I32]{K+,pi-}_phase                     0.0355676
D0[P]{K*(892)0,rho(770)0}_phase                    PiPi40[kMatrix.pole.1]{pi-,pi+}_amp                0.044247
D0[P]{K*(892)0,rho(770)0}_phase                    PiPi40[kMatrix.pole.1]{pi-,pi+}_phase              0.36086
D0[P]{K*(892)0,rho(770)0}_phase                    PiPi40[kMatrix.prod.0]{pi-,pi+}_amp                0.0473402
D0[P]{K*(892)0,rho(770)0}_phase                    PiPi40[kMatrix.prod.0]{pi-,pi+}_phase              0.286271
D0{K(1)(1270)+,pi-}_amp                            D0{K(1)(1270)+,pi-}_phase                          -0.0327894
D0{K(1)(1270)+,pi-}_amp                            D0{K(1)(1400)+{K*(892)0,pi+},pi-}_amp              0.75435
D0{K(1)(1270)+,pi-}_amp                            D0{K(1)(1400)+{K*(892)0,pi+},pi-}_phase            -0.22789
D0{K(1)(1270)+,pi-}_amp                            D0{K*(892)0,rho(1450)0}_amp                        0.258623
D0{K(1)(1270)+,pi-}_amp                            D0{K*(892)0,rho(1450)0}_phase                      -0.204053
D0{K(1)(1270)+,pi-}_amp                            D0{K*(892)0,rho(770)0}_amp                         0.405899
D0{K(1)(1270)+,pi-}_amp                            D0{K*(892)0,rho(770)0}_phase                       -0.118793
D0{K(1)(1270)+,pi-}_amp                            KPi40[FOCUS.I32]{K+,pi-}_amp                       -0.0738693
D0{K(1)(1270)+,pi-}_amp                            KPi40[FOCUS.I32]{K+,pi-}_phase                     -0.116014
D0{K(1)(1270)+,pi-}_amp                            PiPi40[kMatrix.pole.1]{pi-,pi+}_amp                0.436222
D0{K(1)(1270)+,pi-}_amp                            PiPi40[kMatrix.pole.1]{pi-,pi+}_phase              -0.167951
D0{K(1)(1270)+,pi-}_amp                            PiPi40[kMatrix.prod.0]{pi-,pi+}_amp                0.361431
D0{K(1)(1270)+,pi-}_amp                            PiPi40[kMatrix.prod.0]{pi-,pi+}_phase              -0.206115
D0{K(1)(1270)+,pi-}_phase                          D0{K(1)(1400)+{K*(892)0,pi+},pi-}_amp              0.148634
D0{K(1)(1270)+,pi-}_phase                          D0{K(1)(1400)+{K*(892)0,pi+},pi-}_phase            0.636694
D0{K(1)(1270)+,pi-}_phase                          D0{K*(892)0,rho(1450)0}_amp                        -0.0478653
D0{K(1)(1270)+,pi-}_phase                          D0{K*(892)0,rho(1450)0}_phase                      0.205686
D0{K(1)(1270)+,pi-}_phase                          D0{K*(892)0,rho(770)0}_amp                         0.24506
D0{K(1)(1270)+,pi-}_phase                          D0{K*(892)0,rho(770)0}_phase                       0.357408
D0{K(1)(1270)+,pi-}_phase                          KPi40[FOCUS.I32]{K+,pi-}_amp                       0.0628667
D0{K(1)(1270)+,pi-}_phase                          KPi40[FOCUS.I32]{K+,pi-}_phase                     -0.00154524
D0{K(1)(1270)+,pi-}_phase                          PiPi40[kMatrix.pole.1]{pi-,pi+}_amp                -0.0327954
D0{K(1)(1270)+,pi-}_phase                          PiPi40[kMatrix.pole.1]{pi-,pi+}_phase              0.504826
D0{K(1)(1270)+,pi-}_phase                          PiPi40[kMatrix.prod.0]{pi-,pi+}_amp                0.0567432
D0{K(1)(1270)+,pi-}_phase                          PiPi40[kMatrix.prod.0]{pi-,pi+}_phase              0.42393
D0{K(1)(1400)+{K*(892)0,pi+},pi-}_amp              D0{K(1)(1400)+{K*(892)0,pi+},pi-}_phase            -0.021217
D0{K(1)(1400)+{K*(892)0,pi+},pi-}_amp              D0{K*(892)0,rho(1450)0}_amp                        0.33473
D0{K(1)(1400)+{K*(892)0,pi+},pi-}_amp              D0{K*(892)0,rho(1450)0}_phase                      -0.320075
D0{K(1)(1400)+{K*(892)0,pi+},pi-}_amp              D0{K*(892)0,rho(770)0}_amp                         0.430603
D0{K(1)(1400)+{K*(892)0,pi+},pi-}_amp              D0{K*(892)0,rho(770)0}_phase                       -0.0313198
D0{K(1)(1400)+{K*(892)0,pi+},pi-}_amp              KPi40[FOCUS.I32]{K+,pi-}_amp                       -0.0311985
D0{K(1)(1400)+{K*(892)0,pi+},pi-}_amp              KPi40[FOCUS.I32]{K+,pi-}_phase                     -0.14619
D0{K(1)(1400)+{K*(892)0,pi+},pi-}_amp              PiPi40[kMatrix.pole.1]{pi-,pi+}_amp                0.443971
D0{K(1)(1400)+{K*(892)0,pi+},pi-}_amp              PiPi40[kMatrix.pole.1]{pi-,pi+}_phase              -0.0762674
D0{K(1)(1400)+{K*(892)0,pi+},pi-}_amp              PiPi40[kMatrix.prod.0]{pi-,pi+}_amp                0.423165
D0{K(1)(1400)+{K*(892)0,pi+},pi-}_amp              PiPi40[kMatrix.prod.0]{pi-,pi+}_phase              -0.157235
D0{K(1)(1400)+{K*(892)0,pi+},pi-}_phase            D0{K*(892)0,rho(1450)0}_amp                        0.0964794
D0{K(1)(1400)+{K*(892)0,pi+},pi-}_phase            D0{K*(892)0,rho(1450)0}_phase                      0.334818
D0{K(1)(1400)+{K*(892)0,pi+},pi-}_phase            D0{K*(892)0,rho(770)0}_amp                         0.0523969
D0{K(1)(1400)+{K*(892)0,pi+},pi-}_phase            D0{K*(892)0,rho(770)0}_phase                       0.527755
D0{K(1)(1400)+{K*(892)0,pi+},pi-}_phase            KPi40[FOCUS.I32]{K+,pi-}_amp                       -0.0351129
D0{K(1)(1400)+{K*(892)0,pi+},pi-}_phase            KPi40[FOCUS.I32]{K+,pi-}_phase                     0.0360682
D0{K(1)(1400)+{K*(892)0,pi+},pi-}_phase            PiPi40[kMatrix.pole.1]{pi-,pi+}_amp                0.0276071
D0{K(1)(1400)+{K*(892)0,pi+},pi-}_phase            PiPi40[kMatrix.pole.1]{pi-,pi+}_phase              0.465655
D0{K(1)(1400)+{K*(892)0,pi+},pi-}_phase            PiPi40[kMatrix.prod.0]{pi-,pi+}_amp                0.0492405
D0{K(1)(1400)+{K*(892)0,pi+},pi-}_phase            PiPi40[kMatrix.prod.0]{pi-,pi+}_phase              0.364315
D0{K*(892)0,rho(1450)0}_amp                        D0{K*(892)0,rho(1450)0}_phase                      0.0246713
D0{K*(892)0,rho(1450)0}_amp                        D0{K*(892)0,rho(770)0}_amp                         0.00497313
D0{K*(892)0,rho(1450)0}_amp                        D0{K*(892)0,rho(770)0}_phase                       0.313187
D0{K*(892)0,rho(1450)0}_amp                        KPi40[FOCUS.I32]{K+,pi-}_amp                       -0.0390477
D0{K*(892)0,rho(1450)0}_amp                        KPi40[FOCUS.I32]{K+,pi-}_phase                     -0.0843458
D0{K*(892)0,rho(1450)0}_amp                        PiPi40[kMatrix.pole.1]{pi-,pi+}_amp                0.184923
D0{K*(892)0,rho(1450)0}_amp                        PiPi40[kMatrix.pole.1]{pi-,pi+}_phase              -0.0667804
D0{K*(892)0,rho(1450)0}_amp                        PiPi40[kMatrix.prod.0]{pi-,pi+}_amp                0.186887
D0{K*(892)0,rho(1450)0}_amp                        PiPi40[kMatrix.prod.0]{pi-,pi+}_phase              -0.121471
D0{K*(892)0,rho(1450)0}_phase                      D0{K*(892)0,rho(770)0}_amp                         -0.525616
D0{K*(892)0,rho(1450)0}_phase                      D0{K*(892)0,rho(770)0}_phase                       0.148037
D0{K*(892)0,rho(1450)0}_phase                      KPi40[FOCUS.I32]{K+,pi-}_amp                       0.131129
D0{K*(892)0,rho(1450)0}_phase                      KPi40[FOCUS.I32]{K+,pi-}_phase                     0.0563112
D0{K*(892)0,rho(1450)0}_phase                      PiPi40[kMatrix.pole.1]{pi-,pi+}_amp                -0.06408
D0{K*(892)0,rho(1450)0}_phase                      PiPi40[kMatrix.pole.1]{pi-,pi+}_phase              0.320522
D0{K*(892)0,rho(1450)0}_phase                      PiPi40[kMatrix.prod.0]{pi-,pi+}_amp                -0.109427
D0{K*(892)0,rho(1450)0}_phase                      PiPi40[kMatrix.prod.0]{pi-,pi+}_phase              0.297557
D0{K*(892)0,rho(770)0}_amp                         D0{K*(892)0,rho(770)0}_phase                       -0.022271
D0{K*(892)0,rho(770)0}_amp                         KPi40[FOCUS.I32]{K+,pi-}_amp                       -0.0654095
D0{K*(892)0,rho(770)0}_amp                         KPi40[FOCUS.I32]{K+,pi-}_phase                     -0.0566274
D0{K*(892)0,rho(770)0}_amp                         PiPi40[kMatrix.pole.1]{pi-,pi+}_amp                0.193189
D0{K*(892)0,rho(770)0}_amp                         PiPi40[kMatrix.pole.1]{pi-,pi+}_phase              0.0152519
D0{K*(892)0,rho(770)0}_amp                         PiPi40[kMatrix.prod.0]{pi-,pi+}_amp                0.163697
D0{K*(892)0,rho(770)0}_amp                         PiPi40[kMatrix.prod.0]{pi-,pi+}_phase              0.0114896
D0{K*(892)0,rho(770)0}_phase                       KPi40[FOCUS.I32]{K+,pi-}_amp                       0.0244228
D0{K*(892)0,rho(770)0}_phase                       KPi40[FOCUS.I32]{K+,pi-}_phase                     0.0220796
D0{K*(892)0,rho(770)0}_phase                       PiPi40[kMatrix.pole.1]{pi-,pi+}_amp                0.0063992
D0{K*(892)0,rho(770)0}_phase                       PiPi40[kMatrix.pole.1]{pi-,pi+}_phase              0.286132
D0{K*(892)0,rho(770)0}_phase                       PiPi40[kMatrix.prod.0]{pi-,pi+}_amp                0.0248035
D0{K*(892)0,rho(770)0}_phase                       PiPi40[kMatrix.prod.0]{pi-,pi+}_phase              0.209232
KPi40[FOCUS.I32]{K+,pi-}_amp                       KPi40[FOCUS.I32]{K+,pi-}_phase                     -0.070812
KPi40[FOCUS.I32]{K+,pi-}_amp                       PiPi40[kMatrix.pole.1]{pi-,pi+}_amp                -0.302423
KPi40[FOCUS.I32]{K+,pi-}_amp                       PiPi40[kMatrix.pole.1]{pi-,pi+}_phase              0.629195
KPi40[FOCUS.I32]{K+,pi-}_amp                       PiPi40[kMatrix.prod.0]{pi-,pi+}_amp                -0.165137
KPi40[FOCUS.I32]{K+,pi-}_amp                       PiPi40[kMatrix.prod.0]{pi-,pi+}_phase              0.593146
KPi40[FOCUS.I32]{K+,pi-}_phase                     PiPi40[kMatrix.pole.1]{pi-,pi+}_amp                0.577984
KPi40[FOCUS.I32]{K+,pi-}_phase                     PiPi40[kMatrix.pole.1]{pi-,pi+}_phase              0.199319
KPi40[FOCUS.I32]{K+,pi-}_phase                     PiPi40[kMatrix.prod.0]{pi-,pi+}_amp                0.415919
KPi40[FOCUS.I32]{K+,pi-}_phase                     PiPi40[kMatrix.prod.0]{pi-,pi+}_phase              0.0907441
PiPi40[kMatrix.pole.1]{pi-,pi+}_amp                PiPi40[kMatrix.pole.1]{pi-,pi+}_phase              -0.081404
PiPi40[kMatrix.pole.1]{pi-,pi+}_amp                PiPi40[kMatrix.prod.0]{pi-,pi+}_amp                0.865893
PiPi40[kMatrix.pole.1]{pi-,pi+}_amp                PiPi40[kMatrix.prod.0]{pi-,pi+}_phase              -0.313562
PiPi40[kMatrix.pole.1]{pi-,pi+}_phase              PiPi40[kMatrix.prod.0]{pi-,pi+}_amp                0.0741107
PiPi40[kMatrix.pole.1]{pi-,pi+}_phase              PiPi40[kMatrix.prod.0]{pi-,pi+}_phase              0.907965
PiPi40[kMatrix.prod.0]{pi-,pi+}_amp                PiPi40[kMatrix.prod.0]{pi-,pi+}_phase              -0.183979
