# Supplementary material for: Studies of the resonance structure in $D^{0} \to K^\mp \pi^\pm \pi^\pm \pi^\mp$ decays
Source: arXiv:1712.08609 source file (2018-06-18)
Supplement: Supplementary file 2 [file Appendix.tex]

\begin{table}
  
  \begin{tabular}{ll}

    \toprule
    \textbf{Topology} & \textbf{Spin Factor}  \\
    \midrule
    \midrule
    $ \displaystyle P \rightarrow V(P_1 P_2) S(P_3 P_4) $ & $ \displaystyle g_{\mu\nu} L_1(P_V,Q_V)^{\mu} L_1(P_P,Q_P)^{\nu} $ \\
    $ \displaystyle P \rightarrow V_1(P_1 P_2) V_2(P_3 P_4)$ & $ \displaystyle g_{\mu\nu} L_1(P_{V_1},Q_{V_1})^\mu L_1(P_{V_2},Q_{V_2})^\nu $ \\
    $ \displaystyle P \rightarrow [V_1(P_1 P_2) V_2(P_3 P_4)]^{L=1}$
    & $ \displaystyle \varepsilon_{\mu\nu\alpha\beta}{P_P^\mu}  L_{1}^{\nu}(P_P, Q_P ) L_{1}^\mu(P_{V_1}, Q_{V_1} ) L_{1}^\nu(P_{V_2}, Q_{V_2})$ \\
    $ \displaystyle P \rightarrow [V_1(P_1 P_2) V_2(P_3 P_4)]^{L=2}$ & $ \displaystyle L_{2\mu\nu}(P_{V_1}, Q_{V_1} ) L_{1}^\nu(P_{V_2}, Q_{V_2})$ \\
    $ \displaystyle P \rightarrow S_1(P_1 P_2) S_2(P_3 P_4) $ & $ \displaystyle 1 $ \\

    \midrule
    $ \displaystyle P \rightarrow A( V(P_1 P_2 ) P_3 ) P_4 $ & $ \displaystyle L_{1}^{\mu}(P_{P}, Q_{P} ) \mathcal{S}_{\mu\nu}(P_A) L_{1}^{\nu}(P_V,Q_V) $ \\
    $ \displaystyle P \rightarrow V_1( V_2(P_1 P_2 ) P_3 ) P_4 $ &
    $ \displaystyle L_{1}^{\mu}(P_{P}, Q_{P} ) \mathcal{S}_{\mu\nu}(P_V) \varepsilon^{\nu\alpha\beta\gamma}{P_{V\alpha}} \ L_{1\beta}(P_{V_1}, Q_{V_1} ) L_{1\gamma}(P_{V_2},Q_{V_2}) $ \\
    $ \displaystyle P \rightarrow A( V(P_1 P_2 ) P_3 )^{L=2} P_4$ &  $ \displaystyle L_{1}^{\mu}(P_{P}, Q_{P} ) L_{2\mu\alpha}(P_A,Q_A) L_{1}^{\alpha}(P_V,Q_V) $ \\
    $ \displaystyle P \rightarrow T( V(P_1 P_2 ) P_3 )^{L=2} P_4$ & $ \displaystyle L_{2}^{\mu\nu}(P_{P},Q_{P}) \varepsilon_{\mu\gamma\eta\lambda}L_{1\nu}(P_T,Q_T)P_T^{\gamma}Q_T^{\eta}L_1(P_V,Q_V)^{\lambda}$ \\
    \midrule
    $ \displaystyle P \rightarrow P( V(P_1 P_2 ) P_3 ) P_4 $ & $\displaystyle L_{1}^{\mu}(P_P,Q_P)L_{1\mu}(P_V,Q_V)$ \\
    $ \displaystyle P \rightarrow P( S(P_1 P_2 ) P_3 ) P_4 $ & $\displaystyle 1 $ \\

    \bottomrule
  \end{tabular}
  \caption{Spin factors for the topologies used in the amplitude models. Unless otherwise stated, decay products are in their ground-states while obeying relevant conservation laws. Spin factors for amplitudes that are not found to be significant, such as $S\rightarrow TV$ are not tabulated here.}
  \label{tb:TableOfSpinFunctions}

\end{table}
